# Supplementary material for: Influence of the magneto-volume effect on the transient reflectivity of MnSi
Source: arXiv:2402.02174 source file (2024-05-13)
Supplement: Supplementary file 1 [file supplement.pdf]

# Supplemental Material: Ultrafast magneto-volume effect in transient reflectivity measurements of the chiral magnet MnSi

J. Kalin*, S. Sievers, H. W. Schumacher, H. Füser, and M. Bieler

*Physikalisch-Technische Bundesanstalt, 38116 Braunschweig, Germany*

A. Bauer

*Physik-Department, Technische Universität München, 85748 Garching, Germany and*

*Zentrum für QuantumEngineering (ZQE),*

*Technische Universität München, 85748 Garching, Germany*

C. Pfleiderer

*Physik-Department, Technische Universität München, 85748 Garching, Germany*

*Zentrum für QuantumEngineering (ZQE),*

*Technische Universität München, 85748 Garching, Germany and*

*Munich Center for Quantum Science and Technology (MCQST),*

*Technische Universität München, 85748 Garching, Germany*

(*jantje.kalin@ptb.de)

(Dated: February 3, 2024)

This Supplemental Material contains further information on (I) laser heating, (II) the temperature and magnetic field dependence of the transient reflectivity of MnSi, (III) the model used to fit the bipolar transient reflectivity and (IV) the analysis of the magnetic thermal expansion coefficients of MnSi.

## I. ESTIMATION OF LASER HEATING

Subjecting the MnSi sample to femtosecond laser pulses induces an increase in sample temperature across various time scales. In addition to the transient temperature increase occurring at a sub-picosecond scale due to individual femtosecond pulses, the cumulative heat from multiple laser pulses leads to steady-state heating, which we account for when estimating the base temperature.

The transient temperature changes can be phenomenologically characterized using the Three-Temperature-Model [2]. Of special interest in this study is the maximum rise of the spin temperature ($T_s$), as it plays a crucial role in estimating the alteration of magnetic order due to femtosecond laser excitation. However, for an accurate determination of the transient spin temperature, knowledge of the coupling constants between the various heat baths is essential, which are not clear a priori. To establish upper and lower limits for the maximum spin temperature ($T_s$), two coupling scenarios are considered: a) when the energy transfer rate from the electron and phonon to the spin bath ($G_{\mathrm{m}}$) is much larger than the energy transfer rate between electrons and phonons ($G_{\mathrm{ep}}$), and b) when $G_{\mathrm{m}}$ is much smaller than $G_{\mathrm{ep}}$.

In scenario (a), the spins equilibrate with the electrons before the lattice temperature has significantly changed. Consequently, the spin temperature closely mirrors the temporal profile of the electron temperature. The upper limit of the maximum spin temperature ($T_{\mathrm{s,max}}$) in this case is determined by the maximum electron temperature ($T_{\mathrm{e,max}}$) achieved when there is instantaneous energy deposition into the electron bath by the laser pulse. The heat energy $Q$ deposited by the laser pulses in the volume $V$ is dependent on the laser fluence $F$ and the penetration depth $\delta$ and results in an increase of the electron temperature according to the following equation

$$\frac{Q}{V} = \frac{F}{\delta} = \int_{T_{\mathrm{e},0}}^{T_{\mathrm{e,max}}} C_{\mathrm{e}}(T_{\mathrm{e}})dT_{\mathrm{e}}. \tag{S1}$$

Here, $C_{\mathrm{e}}$ represents the specific heat of electrons, defined as $C_{\mathrm{e}} = \gamma_{\mathrm{e}} T_{\mathrm{e}}$, with $\gamma_{\mathrm{e}}$ being the electronic

specific heat coefficient. Consequently, the maximum electron temperature is given by:

$$T_{e,max} = \sqrt{\frac{2F}{\delta\gamma_e} + T_{\mathrm{e},0}^2}, \tag{S2}$$

with $T_{\mathrm{e},0}$ being the sample temperature before laser excitation. This serves as a reasonable approximation for the upper limit of $T_{\mathrm{s,max}}$.

In case (b), $G_\mathrm{m} << G_\mathrm{ep}$, the lattice reaches equilibrium with the electron system before the spin temperature experiences a notable increase. Subsequently, all three subsystems converge to a common temperature denoted as $T_\mathrm{eps}$, representing the maximum spin temperature reached when $G_\mathrm{m}$ is substantially smaller than $G_\mathrm{ep}$ and, thus, the lower limit of $T_{\mathrm{s,max}}$. The equilibrium temperatures of the electron, spin, and lattice can be approximated by considering the heat transfer between the subsystems. In this context, the energy within the electron bath ($Q_\mathrm{e}$) is distributed among the lattice and spin baths based on the specific heat capacities of the respective subsystems ($C_\mathrm{i}$). This distribution is described by the equation:

$$\partial Q_\mathrm{e} = \partial Q_\mathrm{p} + \partial Q_\mathrm{s} \tag{S3}$$

$$\int_{T_{\mathrm{e,max}}}^{T_\mathrm{eps}} C_\mathrm{e}(T_\mathrm{e})dT_\mathrm{e} = \int_{T_0}^{T_\mathrm{eps}} C_\mathrm{p}(T_\mathrm{p})dT_\mathrm{p} + \int_{T_0}^{T_\mathrm{eps}} C_\mathrm{s}(T_\mathrm{s})dT_\mathrm{s}. \tag{S4}$$

To calculate $T_\mathrm{eps}$, we use the specific heat values from Ref. [33] . The spin specific heat $C_\mathrm{s}$ is estimated by substrating the lattice and electron contribution to the specific heat. In the main text $T_{\mathrm{s,max}}$ is given as the mean value of the upper and lower limit of the maximum spin temperature at 10 K and for a laser fluence of $2\,\mu\mathrm{Jcm}^{-2}$. The uncertainty of $T_{\mathrm{s,max}}$ is derived from the standard deviation of the upper and lower limit of the maximum spin temperature.

## II. TEMPERATURE AND MAGNETIC FIELD DEPENDENCE OF THE TRANSIENT REFLECTIVITY OF MNSI

In this section, we provide additional insights into the temperature and magnetic field dependence of the transient reflectivity of MnSi. Figs. S1(a) and (b) show the transient reflectivity measurements of MnSi at 0 T for various temperatures above and below the critical temperature $T_c$. Together with further data this transient reflectivity data was used to determine the amplitude of $\Delta R_m$ in Fig. 3(a) in the main text. We observe a transition from a fast positive to a bipolar transient reflectivity with decreasing temperature as shown in Fig. S1(a). The amplitude of the negative transient increases with decreasing temperature until 29 K, resulting in the observation

of maximum signal at $T_c$. By decreasing the temperature further, as shown in Fig. S1(b), the amplitude of the negative transient decreases.

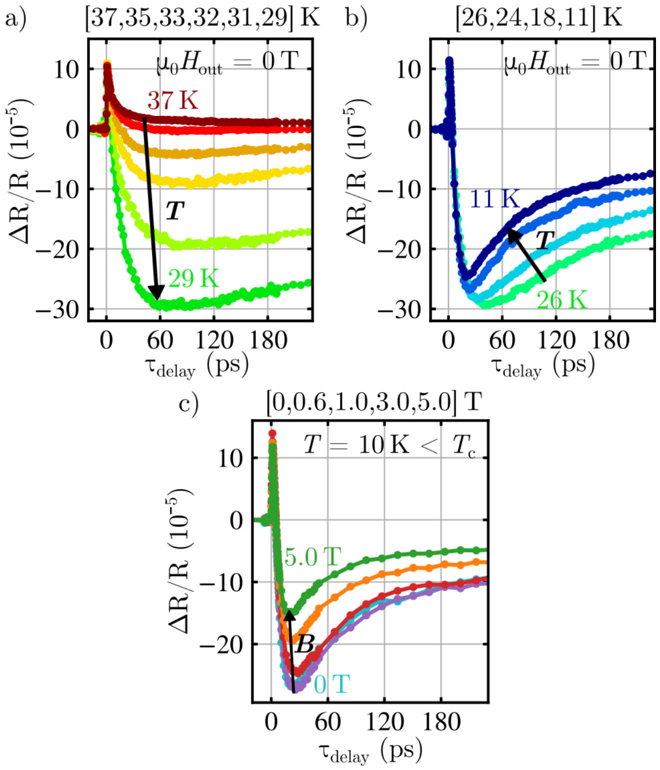


FIG. S1. Temperature and magnetic field dependence of the transient reflectivity of MnSi: a) in the temperature regime from 39 K to 29 K at 0 T, b) from 26 K to 11 K at 0 T and c) at 10 K for various magnetic fields.

Fig. S1(c) shows the transient reflectivity of MnSi for various magnetic fields at $T = 10\,\mathrm{K} < T_c$. This dataset was employed to extract the magnetic field-dependent amplitude of $\Delta R_m$ in Fig. 3(b) in the main text. In the magnetic states below $T_c$, a bipolar transient reflectivity is observed independent of the applied magnetic field. The amplitude of the negative transient decreases with the applied magnetic field. The analysis in the main text attributes this to the diminishing magneto-volume effect for higher magnetic fields due to the saturation of the field-aligned state with the magnetic field.

## III. TRANSIENT REFLECTIVITY MODELLING

In order to analyze the bipolar transient reflectivity we use a phenomenological superposition model. In the main text we show a simplified form to focus on the relevant physics. Here, we present the fitting procedure in full detail. Our model separates the transient reflectivity signal

in two contributions, the non-magnetic thermal $\Delta R_\mathrm{t}$ and magnetic $\Delta R_\mathrm{m}$ contribution. Both are described by an exponential rise and a double exponential decay with different time constants. The non-magnetic reflectivity contribution is modeled by:

$$\Delta R_\mathrm{t}(\tau) = \alpha \cdot (1 - \exp(-\tau/\tau_\mathrm{rise})) \cdot (\exp(-\tau/\tau_\mathrm{ep}) + \exp(-\tau/\tau_\mathrm{th})) \cdot \Theta(\tau) \tag{S5}$$

Here, the $\tau_\mathrm{ep}$ is the electron-phonon thermalization and $\tau_\mathrm{th}$ is the diffusion time constant. The time constant $\tau_\mathrm{rise}$ describes the rise time of the thermal transient. In our model, the magnetic contribution is described by:

$$\Delta R_\mathrm{m}(\tau) = \beta \cdot (1 - \exp(-\tau/\tau_\mathrm{rise,m})) \cdot (\exp(-\tau/\tau_\mathrm{k,m}) + \exp(-\tau/\tau_\mathrm{k,m,2})) \cdot \Theta(\tau). \tag{S6}$$

The rise time of the magnetic transient is given by $\tau_\mathrm{rise,m}$ and the decay times are $\tau_\mathrm{k,m}$ and $\tau_\mathrm{k,m,2}$. The term $\Theta(\tau)$ is an error function (erf) and accounts for the finite width of the probe pulse and the start of excitation at $t = 0$. It is given by:

$$\Theta(\tau) = 0.5 \cdot (1 + \mathrm{erf}(\tau/\tau_L)). \tag{S7}$$

Here, $\tau_L$ is the pulse width of the femtosecond laser.

In Fig. S2 the amplitudes of the thermal and magnetic reflectivity contributions, as determined by the phenomenological model of Eq. (1) in the main text, are shown as a function of temperature for various magnetic fields. The amplitude of $\Delta R_\mathrm{t}$ does not dependent on the applied magnetic field. By increasing the temperature, $\max(\Delta R_\mathrm{t})$ decreases, showing the overall temperature dependence of the reflectivity of MnSi. Apparently, the amplitude of $\Delta R_\mathrm{m}$ shows a different scaling with temperature than $\Delta R_\mathrm{t}$ and peaks around $T_c$. The temperature dependence of the reflectivity also influences $\Delta R_\mathrm{m}(T)$. To account for this and to purely characterize the temperature dependence of the magnetic contribution, we analyze $\Delta \hat{R}_\mathrm{m} = \min(\Delta R_\mathrm{m})/\max(\Delta R_\mathrm{t})$ in the main text. In Fig. S3 we provide further information about the magnetic field dependence of $\Delta \hat{R}_\mathrm{m}$, by presenting data above and below $T_c$. For temperatures above $T_c$, the amplitude of the magnetic transient contribution increases with the applied magnetic field starting at values close to zero. In comparison, below $T_c$, $\Delta \hat{R}_\mathrm{m}$ variates only slightly until $H_\mathrm{c2}$ is reached and decreases afterwards.

## IV. ANALYSIS OF THE MAGNETIC THERMAL EXPANSION COEFFICIENT

For the comparison between the magnetic reflectivity contribution and magneto-volume effect, we take the linear expansion coefficients $\beta = (1/\mathrm{L_0})\mathrm{dL/dT}$ measured with a capacity dilatometer

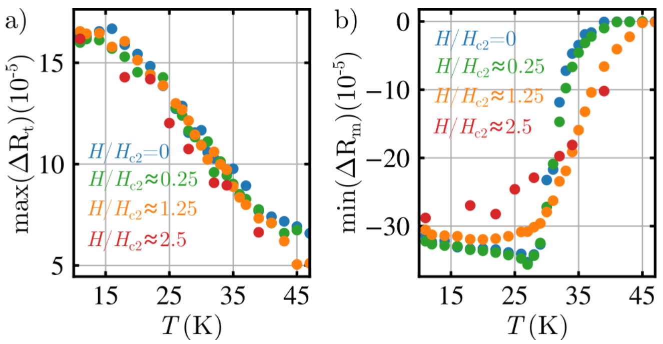


FIG. S2. Temperature dependence of the different contributions to the transient reflectivity of MnSi for various magnetic fields: Amplitude of a) $\Delta R_{\mathrm{t}}$ and (b) $\Delta R_{\mathrm{m}}$.

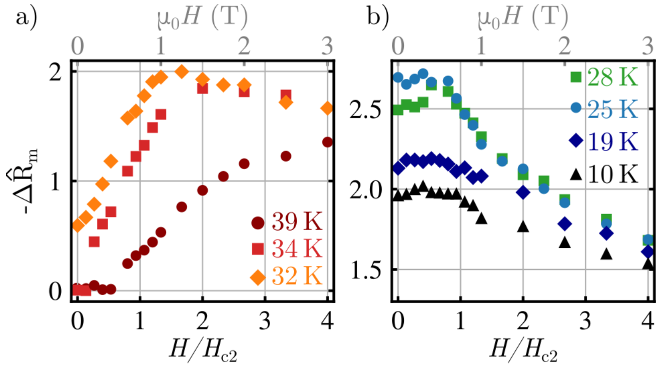


FIG. S3. Amplitude of the magnetic reflectivity transient $\Delta\hat{R}_{\mathrm{m}}$ as a function of the applied magnetic field: a) for $T > T_c$ and b) for for $T < T_c$.

on a comparable MnSi sample from Ref. [19] and [20]. Here, $L_0$ is the sample length at 300 K and dL/dT is the change of sample length with temperature. For the data from Ref. [20] we approximate $\beta$ by $(1/\mathrm{L}_0)(\Delta L(T_2) - \Delta L(T_1))/(T_2 - T_1)$ using measurements of the linear thermal expansion $\Delta L/L_0$ at different temperatures. Thereby, $T_2 - T_1 \approx \Delta T_{\mathrm{s,max}}$.

For the estimation of the magnetic thermal expansion coefficient $\beta_m$, the contribution of the electrons and lattice to the thermal expansion needs to be corrected. To that end, we use the method proposed in Ref. [17]. In this approach, it is assumed that the contributions to $\beta$ from the conduction electrons and lattice are proportional to $T$ and $T^3$, respectively. To eliminate these contributions from $\beta$, we plot $\beta/T$ against $T^2$ as shown in Fig. S4(a). As anticipated, above $T_c$ a linear relation between $\beta/T$ and $T^2$ is observed, which we quantify by a least square fit $\beta/T = a + bT^2$ to the plotted data, yielding $a = 5.5 \cdot 10^{-8}\mathrm{K}^{-2}$ and $b = 8.7 \cdot 10^{-13}\mathrm{K}^{-4}$ as fit parameters (see Fig. S4(a)). Thus, by subtracting $aT + bT^3$ from $\beta$ the magnetic expansion coefficient $\beta_m$,

which is caused by the magneto-volume effect, can be extracted. This is shown exemplarily for 0 T in Fig. S4(b). The magnetic expansion coefficient is zero for $T >> T_c$, as expected. Note here, that the lattice and phonon contributions could not be extracted in the case of magnetic field dependent $\beta$ data from Ref. [20], as the required temperature dependent data is missing. In this case, we use the corrections determined from the temperature dependent measurements from Ref. [19] at 0 T.

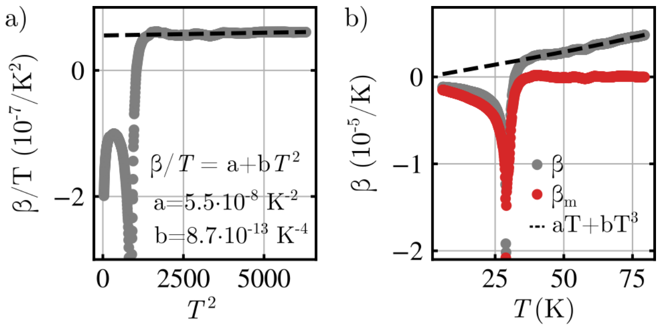


FIG. S4. Estimation of the magnetic thermal expansion coefficient: a) $\beta/T$ versus $T^2$ plot of the thermal expansion at zero magnetic field. The dashed line is the least square fit $\beta/T = a + bT$ to the data above $T_c$. b) Thermal expansion coefficient of MnSi and its magnetic contribution as a function of temperature. The dashed line represents the electron and lattice contribution to the thermal expansion.
